# Supplementary material for: Predicting Economic Development using Geolocated Wikipedia Articles
Source: arXiv:1905.01627 source file (2019-05-11)
Supplement: Supplementary file 1 [file 0_supplement.tex]

\section{Supplementary Work}

\subsection{Wiki Embedding Model}
To robustly understand the impact of cross-national boundary predictions, we further analyze the spearman rho squared results of our cross-national boundary predictions. This allows us to better qualify how the model ranks relative wealth between Wikipedia embeddings. 

%\begin{figure}[H]
%    \begin{subfigure}{.5\textwidth}
%        \centering
%        \includegraphics[width=3.0in]{diagram/wiki_spearman.png}
%    \end{subfigure}
%    \begin{subfigure}{.5\textwidth}
%        \centering
%        \includegraphics[width=3.0in]{diagram/wiki_africa_transfer.png}
%    \end{subfigure}
%    \label{fig:Spearman Doc2Vec}
%    \caption{\textbf{Top: }Spearman's $\rho^2$ - Wikipedia Embedding model trained on column country and tested on row country. \textbf{Bottom: }Plot of Predicted vs. Observed Rank for Wikipedia Embedding model trained on Nigeria and tested on the rest of Africa.}
%\end{figure}

\subsection{Error Analysis}
We perform additional error analysis to identify the root cause of errors in the predictions of our model. We find that the model is unable to differentiate in fine-grained areas with poverty values in a wide range. We hypothesize that this confusion is caused by the data jitter. Another explanation is due to the dataset creation. The nightlight images are over a 5km x 5km area which in clustered datapoints would result in majority of the images being very similar. Further, since we use the closest 10 articles, there may be significant overlap. 

\begin{figure}[H]
\centering
\includegraphics[width=3in]{diagram/nigeria-zimbabwe-pred.png}
\caption{Visualization of results trained on Nigeria, tested on Zimbabwe for Wikipedia Embedding + Nightlight Summary -- Note that the model is unable to have a fine-grained differentiation on certain points. The jitter confuses the model's prediction on certain coordinates. }
\label{fig:Error Viz}
\end{figure}

Interestingly, for many of our models the rank differences result in a normal distribution, with majority of the ranks being predicted as correct.

\begin{figure}[H]
\centering
\includegraphics[width=3.4in]{diagram/CNN-example-hist.png}
\caption{Sample Rank difference distribution for Wikipedia Embedding + Nightlights model}
\end{figure}
